# Supplementary material for: Learning Compositional Neural Programs with Recursive Tree Search and Planning
Source: arXiv:1905.12941 source file (2021-04-13)
Supplement: Supplementary file 1 [file appendix.tex]

\section*{Appendix}
\subsection{Teacher forcing}
When learning higher level programs a major difficulty arises from the fact that lower level programs might still not execute correctly, i.e. lead to a wrong environment state. It leads to very unstable training and often results in failure. Thus, when learning programs of levels higher than 1, we use a teacher forcing strategy. To do so, we assume that we have an oracle that can set the environment in a correct final state for a given program. When lower level programs are called, instead of executing them we directly put the environment in a correct final state, since we have this information, thus imitating the correct program behavior. At the end of the training, we evaluate the program performance without teacher forcing. The use of teacher forcing is for the moment one of the most important element to train the AlphaNPI. The oracle assumption might seem strong however this information is often available, especially in robotics applications.

\subsection{Towards robotic applications}
We believe that one major application field for our NPI algorithm might be robotics. Let us consider an example. A robot is to clean a room, i.e. taking objects that are misplaced and moving them to their right place. Let us imagine that we have previously trained deep rl agents on continuous action spaces (with an algorithm such as TD3, PPO or SAC for instance) to perform the following tasks:

\begin{table}[h!]
\centering
\begin{tabular}{|l|c|}
\hline
\textbf{task} & \textbf{policy name} \\
\hline
take object  &   $\pi_{\theta_1}$ \\
drop object & $\pi_{\theta_2}$ \\
walk &  $\pi_{\theta_3}$ \\
look around & $\pi_{\theta_4}$\\
\hline
\end{tabular}
\end{table}

We can use these primary policies to define level zero programs and from this programs define a whole library of programs in our AlphaNPI formulation.\\

\begin{table}[h!]
\centering
\begin{tabular}{|l|l|c|}
\hline
\textbf{program} & \textbf{definition} & \textbf{level} \\
\hline
Take\_Object() & call $\pi_{\theta_1}$ for $n_1$ time steps & 0\\
Drop\_Object() & call $\pi_{\theta_2}$ for $n_2$ time steps & 0\\
Walk() & call $\pi_{\theta_3}$ for $n_3$ time steps & 0\\
Look\_Around() & call $\pi_{\theta_4}$ for $n_4$ time steps & 0\\
\hline
Move\_Object() & move an object in the room & 1\\
Find\_Next\_Object() & find the next object to move & 1\\
\hline
Clean\_Room() & move all objects to their correct place & 2\\
\hline
\end{tabular}
\end{table}
In this setting, the AlphaNPI role is to find when to call and how many times to call the already trained deep rl agents in order to solve one or several global tasks. During the AlphaNPI training, the experience collected might be reused as well to keep training the deep rl agents. 

\subsection{PUCT criteria}
\begin{equation}
    U([i_t, e_t], a) = c_{puct}P([i_t, e_t], a)\dfrac{\sqrt{\sum_b N([e_t, i_t], b)}}{1 + N([e_t, i_t], a)}
\end{equation}
